# Supplementary material for: An Improved Self-supervised GAN via Adversarial Training
Source: arXiv:1905.05469 source file (2019-05-14)
Supplement: Supplementary file 1 [file supp.tex]

In this supplementary material, we provide further analysis of our proposed techniques: (i) We compare our performance to the state-of-the-art conditional GAN, SAGAN \cite{zhang-arxiv-2018} (ii) We integrate our techniques into SSGAN baseline \cite{chen-arxiv-2018} to analyze their influence, and (iii) We describe the network architectures that we used in our studies and experiments.

\section{Comparing to conditional GAN}

We analyze the effectiveness of our proposed model via comparing to the state-of-the-art conditional GAN, SAGAN \cite{zhang-arxiv-2018}. We modify its published code\footnote{https://github.com/brain-research/self-attention-gan} and change the ResNet architecture similar to \cite{gulrajani-arxiv-2017} to train SAGAN on CIFAR-10 dataset. We set up this experiment in the same conditions as our model. We observe that although SAGAN is conditional, it is not always stable on CIFAR-10. For example, it often diverges from iteration 200K. To be comparable, we run SAGAN four times and compute the average FID scores at the iteration 200K of these runs. FID is computed with 10K-5K. The average FID of SAGAN is $14.59 \pm 1.04$, which is similar to the FID of our best setting ($14.75$ in Table 1 of our main manuscript) with the same ResNet architecture. Note that the performance of our model (SS) (14.97 in Table 1 of our main manuscript) is also similar to SAGAN. In other words, our model (SS) achieves the saturated performance, because SAGAN can be seen as the bound of unconditional GAN for the same specific network. Therefore, it's hard to improve it further significantly although being combined with adversarial training and our generator objective. Moreover, our model does not suffer the divergence issue with ResNet architecture like SAGAN. This experiment again confirms the robustness and stability of our proposed model. Note that we cannot do the same with STL-10 because it does not have labels for all 100K training images. Yet, we believe that the result of STL-10 is saturated either on the current network capacity, therefore it's hard to improve it further.

\section{Improving SSGAN baseline}

We analyze the effectiveness of our proposed techniques as we integrate them into the SSGAN method \cite{chen-arxiv-2018}. In particular, we replace its objectives and our proposed objectives to understand their influence.

First, we verify the SSGAN baseline. We use the similar DCGAN architecture as in our main manuscript (see Section \ref{network-architecture} of this supplementary material). The results of this study are presented in Fig. \ref{ssgan-baseline}. We fix $\lambda_d = 1.0$, and fine-tune $\lambda_g$. The results show that $\lambda_g = 0.2$ is the best, which is the same as suggested in the original paper \cite{chen-arxiv-2018}. We then add the adversarial training to the classifier of SSGAN like our method (+ adversarial), but the result gets worse (SSGAN + adversarial) than non-adversarial version. This result does not suggest to apply adversarial training for the classifier of original SSGAN. In other words, the generator objective (the classification task) of SSGAN is unable to be combined with adversarial training of the classifier.

Then, we replace the classification task of generator objective (Eq. 6 in our manuscript) -- referred as Entropy-Matching here -- to that of SSGAN and then fine-tune $\lambda_g$ for this term with adversarial training for discriminator (classification task). We find that $\lambda_g = 0.1$ is the best with Entropy-Matching, which is consistent with our proposed model as using the same DCGAN architecture (Fig. 2 of our main manuscript). Fig. \ref{ssgan-baseline} show that using our proposed generator objective is better than using the original ones of SSGAN (with the best choice of $\lambda_g$ for both). Importantly, the classification task of our generator objective likely supports the adversarial training of the classifier. The FID of our version (SSGAN + Entropy-Matching) is significantly improved when we add the adversarial training for the classifier (SSGAN + Entropy-Matching + adversarial). Although it diverges at the end, this result shows good effects of our proposed techniques to standard GAN. Moreover, it explains why we choose the auto-encoder based method, Dist-GAN \cite{tran-eccv-2018}, as the baseline in our work. It is more stable to get benefits from our proposed techniques of self-supervised training (to significantly improve the FID and without suffering the divergence issue). It again confirms that the combination of our classification task (of generator objective) and the adversarial training of classifier boosts the FID of the GAN model significantly. In addition, when we combine multiple constraints in a good way (Dist-GAN + our proposed techniques), the GAN model gets much more stable and achieves the state-of-the-art FID scores of unconditional GAN.

\begin{figure}
\centering
\includegraphics[scale=0.3]{figs/cifar_dcgan_ss_gan_compare}
\caption{The FID by SSGAN baseline and versions as our techniques are integrated (+ Entropy-Matching or + adversarial). We fix $\lambda_d = 1.0$ and fine-tune $\lambda_g$.}
\label{ssgan-baseline}
\end{figure}

\section{Network Architectures}
\label{network-architecture}

\subsection{DCGAN}

Our DCGAN architecture, which is used for ablation studies on CIFAR-10, are presented in Table. \ref{dcgan}.

\begin{table}[ht!]
	\caption{\label{dcgan}Our DCGAN architecture is similar to \cite{radford-arxiv-2015} but the smaller number of feature maps (D = 64) to be more efficient for our ablation study on CIFAR-10. The Encoder is the mirror of the Generator. Slopes of lReLU functions are set to $0.2$. $\mathcal{U}(0, 1)$ is the uniform distribution.}
   	\centering
   	\small
    \begin{subtable}{.32\linewidth}
    	\centering
    	{\begin{tabular}{c}
			\toprule
			\midrule
		 	RGB image $x\in \bbR^{M\times M \times 3}$ \\
            \midrule
            5$\times$5, stride=2 conv. 1 $\times$ D ReLU\\
            \midrule
            5$\times$5, stride=2 conv. BN 2 $\times$ D ReLU\\        		 	
			\midrule
            5$\times$5, stride=2 conv. BN 4 $\times$ D ReLU\\            	
            \midrule
            5$\times$5, stride=2 conv. BN 8 $\times$ D ReLU\\    
            \midrule          
            dense $\rightarrow$ 128 \\
            \midrule
			\bottomrule
		\end{tabular}}
        \caption{\label{tab:enc_dcgan}Encoder, $M=32$ for CIFAR-10}
    \end{subtable}   	
    \begin{subtable}{.32\linewidth}
    	\centering
    	{\begin{tabular}{c}
			\toprule
			\midrule
		 	$z\in \bbR^{128} \sim \mathcal{U}(0, 1)$ \\	 	
           	\midrule
            dense $\rightarrow$ 2 $\times$ 2 $\times$ 8 $\times$ D  \\
            \midrule
            5$\times$5, stride=2 deconv. BN 4 $\times$ D ReLU\\
			\midrule
            5$\times$5, stride=2 deconv. BN 2 $\times$ D ReLU\\
            \midrule
            5$\times$5, stride=2 deconv. BN 1 $\times$ D ReLU\\
            \midrule
            5$\times$5, stride=2 deconv. 3 Sigmoid\\	
            \midrule
			\bottomrule
		\end{tabular}}
        \caption{\label{tab:gen_dcgan}Generator for CIFAR-10}
    \end{subtable}
    \begin{subtable}{.34\linewidth}
    	\centering
    	{\begin{tabular}{c}
			\toprule
			\midrule
			RGB image $x\in \bbR^{M\times M \times 3}$ \\
            \midrule
            5$\times$5, stride=2 conv. 1 $\times$ D lReLU\\
            \midrule
            5$\times$5, stride=2 conv. BN 2 $\times$ D lReLU\\        		 	
			\midrule
            5$\times$5, stride=2 conv. BN 4 $\times$ D lReLU\\            	
            \midrule
            5$\times$5, stride=2 conv. BN 8 $\times$ D lReLU\\    
            \midrule
            dense $\rightarrow$ 1, dense $\rightarrow$ 5 (two heads) \\
            \midrule
			\bottomrule
		\end{tabular}}
        \caption{\label{tab:dis_dcgan}Discriminator, $M=32$ for CIFAR-10. Two heads for the real/fake discriminator and multi-class classifier.}
    \end{subtable}
\end{table}

\subsection{SNGAN}

Our SN-GAN architectures for CIFAR-10 and STL-10 datasets are presented in Table. \ref{tab:sngan_models}.

\begin{table}[ht!]
	\caption{\label{tab:sngan_models} Encoder, generator, and discriminator of standard CNN architectures for CIFAR-10 and STL-10 used in our experiments. We use similar architectures as ones in \cite{miyato-iclr-2018}. The Encoder is the mirror of the Generator. Slopes of lReLU functions are set to $0.1$. $\mathcal{U}(0, 1)$ is the uniform distribution.}
   	\centering
   	\small
    \begin{subtable}{.33\linewidth}
    	\centering
    	{\begin{tabular}{c}
			\toprule
			\midrule
		 	RGB image $x\in \bbR^{M\times M \times 3}$ \\
            \midrule
            3$\times$3, stride=1 conv. 64\\	
            \midrule
            4$\times$4, stride=2 conv. BN 128 ReLU\\            		 	
			\midrule
            4$\times$4, stride=2 conv. BN 256 ReLU\\           	
            \midrule
            4$\times$4, stride=2 conv. BN 512 ReLU\\  
            \midrule          
            dense $\rightarrow$ 128 \\
            \midrule
			\bottomrule
		\end{tabular}}
        \caption{\label{tab:enc}Encoder, $M=32$ for CIFAR-10, and $M=48$ for STL-10}
    \end{subtable}   	
    \begin{subtable}{.33\linewidth}
    	\centering
    	{\begin{tabular}{c}
			\toprule
			\midrule
		 	$z\in \bbR^{128} \sim \mathcal{U}(0, 1)$ \\	 	
           	\midrule
            dense $\rightarrow$ $M_g$ $\times$ $M_g$ $\times$ 512 \\
            \midrule
            4$\times$4, stride=2 deconv. BN 256 ReLU\\
			\midrule
            4$\times$4, stride=2 deconv. BN 128 ReLU\\
            \midrule
            4$\times$4, stride=2 deconv. BN 64 ReLU\\
            \midrule
            3$\times$3, stride=1 conv. 3 Sigmoid\\	
            \midrule
			\bottomrule
		\end{tabular}}
        \caption{\label{tab:gen}Generator, $M_g=4$  for CIFAR-10, and $M_g=6$ for STL-10}
    \end{subtable}
    \begin{subtable}{.32\linewidth}
    	\centering
    	{\begin{tabular}{c}
			\toprule
			\midrule
		 	RGB image $x\in \bbR^{M\times M \times 3}$ \\
			\midrule
            3$\times$3, stride=1 conv 64 lReLU\\
            4$\times$4, stride=2 conv 64 lReLU\\
            \midrule
            3$\times$3, stride=1 conv 128 lReLU\\
            4$\times$4, stride=2 conv 128 lReLU\\
            \midrule
            3$\times$3, stride=1 conv 256 lReLU\\
            4$\times$4, stride=2 conv 256 lReLU\\
            \midrule
            3$\times$3, stride=1 conv. 512 lReLU\\
            \midrule
            dense $\rightarrow$ 1, dense $\rightarrow$ 5 (two heads)\\
			\bottomrule
		\end{tabular}}
        \caption{\label{tab:dis_deep}Discriminator, $M=32$ for CIFAR-10, and $M=48$ for STL-10. Two heads for the real/fake discriminator and multi-class classifier.}
    \end{subtable}
\end{table}

\subsection{ResNet}

Our ResNet architectures for CIFAR-10 and STL-10 are presented in Table. \ref{tab:resnets_cifar10} and Table. \ref{tab:resnets_stl}.

\begin{figure}[ht!]
	\begin{tabular}{cc}
	     \small
        \begin{minipage}{1.\textwidth}
          \tblcaption{\label{tab:resnets_cifar10}ResNet architecture for CIFAR10 dataset. The Encoder is the mirror of the Generator. We use similar architectures and ResBlock to the ones used in \cite{miyato-iclr-2018}. $\mathcal{U}(0, 1)$ is the uniform distribution.}
          \centering
          \begin{subtable}{.33\textwidth}
                        \centering
                        {\begin{tabular}{c}
                            \toprule
                            \midrule
                            RGB image $x\in \bbR^{32\times 32 \times 3}$ \\
                            \midrule
                            3$\times$3 stride=1, conv. 256\\ 
                            \midrule
                            ResBlock down 256\\                
                            \midrule
                            ResBlock down 256\\
                            \midrule
                            ResBlock down 256\\                                                                   
                            \midrule
                            dense $\rightarrow$ 128 \\
                            \midrule
                            \bottomrule
                        \end{tabular}}
                        \caption{Encoder}
                    \end{subtable}
          \begin{subtable}{.33\textwidth}
              \centering
              {\begin{tabular}{c}
                  \toprule
                  \midrule
                  $z\in \bbR^{128} \sim \mathcal{U}(0, 1)$ \\
                  \midrule
                  dense, $4 \times 4 \times 256$ \\
                  \midrule
                  ResBlock up 256\\
                  \midrule
                  ResBlock up 256\\
                  \midrule
                  ResBlock up 256\\
                  \midrule
                  BN, ReLU, 3$\times$3 conv, 3 Sigmoid\\
                  \midrule
                  \bottomrule
              \end{tabular}}
              \caption{Generator}
          \end{subtable}
          \begin{subtable}{.32\textwidth}
              \centering
              {\begin{tabular}{c}
                  \toprule
                  \midrule
                  RGB image $x\in \bbR^{32\times 32 \times 3}$ \\
                  \midrule
                  ResBlock down 128\\
                  \midrule
                  ResBlock down 128\\
                  \midrule
                  ResBlock 128\\
                  \midrule
                  ResBlock 128\\
                  \midrule
                  ReLU\\
                  \midrule
                  Global sum pooling\\
                  \midrule
                  dense $\rightarrow$ 1, dense $\rightarrow$ 5 (two heads)\\
                  \midrule
                  \bottomrule
              \end{tabular}}
              \caption{Discriminator. Two heads for the real/fake discriminator and multi-class classifier.}
          \end{subtable}
        \end{minipage}
    \end{tabular}
\end{figure}

\begin{table}[ht!]
          \caption{\label{tab:resnets_stl}ResNet architecture for STL-10 dataset. The Encoder is the mirror of the Generator. We use similar architectures and ResBlock to the ones used in \cite{miyato-iclr-2018}. $\mathcal{U}(0, 1)$ is the uniform distribution.}
          \centering
          \small
          \begin{subtable}{.33\textwidth}
                        \centering
                        {\begin{tabular}{c}
                            \toprule
                            \midrule
                            RGB image $x\in \bbR^{48\times 48 \times 3}$\\
                            \midrule
                            3$\times$3 stride=1, conv. 64\\                            
                            \midrule
                            ResBlock down 128\\
                            \midrule 
                            ResBlock down 256\\
                            \midrule 
                            ResBlock down 512\\
                            \midrule                                 
                            dense $\rightarrow$ 128 \\
                            \midrule
                            \bottomrule
                        \end{tabular}}
                        \caption{Encoder}
                    \end{subtable}
          \begin{subtable}{.33\textwidth}
              \centering
              {\begin{tabular}{c}
                  \toprule
                  \midrule
                  $z\in \bbR^{128} \sim \mathcal{U}(0, 1)$ \\
                  \midrule
                  dense, $6 \times 6 \times 512$ \\
                  \midrule
                  ResBlock up 256\\
                  \midrule
                  ResBlock up 128\\
                  \midrule
                  ResBlock up 64\\
                  \midrule
                  BN, ReLU, 3$\times$3 conv, 3 Sigmoid\\
                  \midrule
                  \bottomrule
              \end{tabular}}
              \caption{Generator}
          \end{subtable}
          \begin{subtable}{.32\textwidth}
              \centering
              {\begin{tabular}{c}
                  \toprule
                  \midrule
                  RGB image $x\in \bbR^{48\times 48 \times 3}$ \\
                  \midrule
                  ResBlock down 64\\
                  \midrule
                  ResBlock down 128\\
                  \midrule
                  ResBlock down 256\\
                  \midrule
                  ResBlock down 512\\
                  \midrule
                  ResBlock 1024\\
                  \midrule
                  ReLU\\
                  \midrule
                  Global sum pooling\\
                  \midrule
                  dense $\rightarrow$ 1, dense $\rightarrow$ 5 (two heads)\\
                  \midrule
                  \bottomrule
              \end{tabular}}
              \caption{Discriminator. Two heads for the real/fake discriminator and multi-class classifier.}
          \end{subtable}
\end{table}
